# Supplementary material for: A Survey on Vertical Federated Learning: From a Layered Perspective
Source: arXiv:2304.01829 source file (2023-04-04)
Supplement: Supplementary file 1 [file appendix.tex]

\newpage
\appendices
\section{Existing Works}

\begin{table*}[!t]
\caption{Main contribution of existing vertical federated learning works.}
%\label{tab:contribution}
\centering
\begin{tabularx}{0.8\linewidth}{cc}
\toprule
Main contribution & Existing vertical federated learning works \\
\midrule
Federated learning algorithm & \makecell[c]{
	\textcolor[rgb]{0.26,0.44,0.76}{Gasc{\'o}n~\textit{et al.}, 2017~\cite{gascon2017privacy}};
	\textcolor[rgb]{0.26,0.44,0.76}{khodaparast~\textit{et al.}, 2018~\cite{khodaparast2018privacy}};
	\textcolor[rgb]{0.26,0.44,0.76}{Feng~\textit{et al.}, 2019~\cite{feng2019securegbm}}; \\
	\textcolor[rgb]{0.26,0.44,0.76}{Gu~\textit{et al.}, 2020~\cite{gu2020federated}};
	\textcolor[rgb]{0.26,0.44,0.76}{Dang~\textit{et al.}, 2020~\cite{dang2020large}};
	\textcolor[rgb]{0.26,0.44,0.76}{Wu~\textit{el al.}, 2020~\cite{wu2020privacy}}; \\
	\textcolor[rgb]{0.26,0.44,0.76}{Ou~\textit{et al.}, 2020~\cite{ou2020homomorphic}};
	\textcolor[rgb]{0.66,0.81,0.55}{Tian~\textit{et al.}, 2020~\cite{tian2020federboost}};
	\textcolor[rgb]{0.66,0.81,0.55}{Cheung and Yu, 2020~\cite{cheung2020federated}}; \\
	\textcolor[rgb]{0.26,0.44,0.76}{Cheng~\textit{el al.}, 2021~\cite{cheng2021secureboost}};
	\textcolor[rgb]{0.26,0.44,0.76}{Kyohei and Masakazu, 2021~\cite{atarashi2021vertical}};
	\textcolor[rgb]{0.26,0.44,0.76}{Fu~\textit{et al.}, 2021~\cite{fu2021vf2boost}}; \\
	\textcolor[rgb]{0.26,0.44,0.76}{Kholod~\textit{et al.}, 2021~\cite{kholod2021parallelization}};
	\textcolor[rgb]{0.66,0.81,0.55}{Ni~\textit{et al.}, 2021~\cite{ni2021vertical}};
	\textcolor[rgb]{0.66,0.81,0.55}{Chu and Zhang, 2021~\cite{chu2021privacy}}; \\
	\textcolor[rgb]{0.66,0.81,0.55}{Che~\textit{et al.}, 2021~\cite{che2021federated}};
	\textcolor[rgb]{0.66,0.81,0.55}{Zhang~\textit{et al.}, 2021~\cite{zhang2021federated}};
	\textcolor[rgb]{0.66,0.81,0.55}{Liang~\textit{et al.}, 2021~\cite{liang2021self}}} \\
\midrule
Federated framework & \makecell[c]{
    \textcolor[rgb]{0.26,0.44,0.76}{Gupta and Raskar, 2018~\cite{gupta2018distributed}};
    \textcolor[rgb]{0.66,0.81,0.55}{Vepakomma~\textit{et al.}, 2018~\cite{vepakomma2018split}}
	\textcolor[rgb]{0.26,0.44,0.76}{Hu~\textit{et al.}, 2019~\cite{hu2019fdml}}; \\
	\textcolor[rgb]{0.26,0.44,0.76}{Yang~\textit{et al.}, 2019~\cite{yang2019federated}};
	\textcolor[rgb]{0.92,0.49,0.19}{Liu~\textit{et al.}, 2019~\cite{liu2019communication}};
	\textcolor[rgb]{0.92,0.49,0.19}{Yang~\textit{et al.}, 2019~\cite{yang2019parallel}}; \\
	\textcolor[rgb]{0.66,0.81,0.55}{Hu~\textit{et al.}, 2019~\cite{hu2019learning}};
	\textcolor[rgb]{0.66,0.81,0.55}{Singh~\textit{et al.}, 2019~\cite{singh2019detailed}};
    \textcolor[rgb]{0.26,0.44,0.76}{Li~\textit{et al.}, 2020~\cite{li2020efficient}}; \\
    \textcolor[rgb]{0.26,0.44,0.76}{Liu~\textit{et al.}, 2020~\cite{liu2020federated}};
    \textcolor[rgb]{0.92,0.49,0.19}{Zhang~\textit{et al.}, 2020~\cite{zhang2020vertical}};
	\textcolor[rgb]{0.92,0.49,0.19}{Chen~\textit{et al.}, 2020~\cite{chen2020vafl}}; \\
	\textcolor[rgb]{0.92,0.49,0.19}{Li~\textit{et al.}, 2020~\cite{li2021label}};
	\textcolor[rgb]{0.66,0.81,0.55}{Feng and Yu, 2020~\cite{feng2020multi}}; \\
	\textcolor[rgb]{0.66,0.81,0.55}{Hu~\textit{et al.}, 2020~\cite{hu2020oarf}};
	\textcolor[rgb]{0.66,0.81,0.55}{Ceballos~\textit{et al.}, 2020~\cite{ceballos2020splitnn}};
	\textcolor[rgb]{0.66,0.81,0.55}{Tajeddine~\textit{et al.}, 2020~\cite{tajeddine2020privacy}}; \\
	\textcolor[rgb]{0.26,0.44,0.76}{Gu~\textit{et al.}, 2021~\cite{gu2021privacy}};
	\textcolor[rgb]{0.26,0.44,0.76}{Wei~\textit{et al.}, 2021~\cite{wei2021privacy}};
	\textcolor[rgb]{0.26,0.44,0.76}{Zhang~\textit{et al.}, 2021~\cite{zhang2021secure}}; \\
	\textcolor[rgb]{0.26,0.44,0.76}{Yang~\textit{et al.}, 2021~\cite{yang2021model}};
	\textcolor[rgb]{0.26,0.44,0.76}{Cha~\textit{et al.}, 2021~\cite{cha2021implementing}};
	\textcolor[rgb]{0.26,0.44,0.76}{Zhou~\textit{et al.}, 2021~\cite{zhou2021privacy}}; \\
	\textcolor[rgb]{0.26,0.44,0.76}{Das and Patterson, 2021~\cite{das2021multi}};
	\textcolor[rgb]{0.92,0.49,0.19}{Romanini~\textit{et al.}, 2021~\cite{romanini2021pyvertical}};
	\textcolor[rgb]{0.92,0.49,0.19}{Chen~\textit{et al.}, 2021~\cite{chen2021fed}}; \\
	\textcolor[rgb]{0.66,0.81,0.55}{Xia~\textit{et al.}, 2021~\cite{xia2021vertical}}; 
	\textcolor[rgb]{0.66,0.81,0.55}{Song and Shen, 2021~\cite{wenjie2021vertical}};
	\textcolor[rgb]{0.66,0.81,0.55}{Mugunthan~\textit{et al.}, 2021~\cite{mugunthan2021multi}}; \\
	\textcolor[rgb]{0.66,0.81,0.55}{Avelar~\textit{et al.}, 2021~\cite{Avelar2021VerticalFL}};
	\textcolor[rgb]{0.66,0.81,0.55}{Xu~\textit{et al.}, 2021~\cite{xu2021fedv}};
	\textcolor[rgb]{0.26,0.44,0.76}{Zhang~\textit{et al.}, 2021~\cite{zhang2021asysqn}};} \\
\midrule
Optimization method & \makecell[c]{
	\textcolor[rgb]{0.26,0.44,0.76}{Hu and Klabjan, 2017~\cite{nathan2017optimization}};
    \textcolor[rgb]{0.92,0.49,0.19}{Yang~\textit{et al.}, 2019~\cite{yang2019quasi}};
    \textcolor[rgb]{0.66,0.81,0.55}{Zheng~\textit{et al.}, 2020~\cite{zheng2020vertical}}; \\
    \textcolor[rgb]{0.66,0.81,0.55}{Song and Shen, 2021~\cite{wenjie2021vertical}}} \\
\midrule
Incentive mechanism & \makecell[c]{
	\textcolor[rgb]{0.26,0.44,0.76}{Wang~\textit{et al.}, 2019~\cite{wang2019measure}};
	\textcolor[rgb]{0.66,0.81,0.55}{Wang, 2019~\cite{wang2019interpret}}} \\
\midrule
System \& network & \makecell[c]{
	\textcolor[rgb]{0.92,0.49,0.19}{Liu, 2020~\cite{liu2020accelerating}};
    \textcolor[rgb]{0.92,0.49,0.19}{Yang~\textit{et al.}, 2020~\cite{yang2020fpga}}}\\
\midrule
Entity alignment & \makecell[c]{
	\textcolor[rgb]{0.66,0.81,0.55}{Hardy~\textit{et al.}, 2017~\cite{hardy2017private}};
    \textcolor[rgb]{0.66,0.81,0.55}{Nock~\textit{et al.}, 2018~\cite{nock2018entity}};
    \textcolor[rgb]{0.26,0.44,0.76}{Lu and Ding, 2020~\cite{lu2020multi}}; \\
    \textcolor[rgb]{0.92,0.49,0.19}{Kang~\textit{et al.}, 2020~\cite{kang2022fedcvt}};
    \textcolor[rgb]{0.92,0.49,0.19}{Liu~\textit{et al.}, 2020~\cite{liu2020asymmetrically}};
    \textcolor[rgb]{0.66,0.81,0.55}{Angelou~\textit{et al.}, 2020~\cite{angelou2020asymmetric}}; \\
    \textcolor[rgb]{0.66,0.81,0.55}{Sun~\textit{et al.}, 2020~\cite{sun2021vertical}};
    \textcolor[rgb]{0.26,0.44,0.76}{Nock~\textit{et al.}, 2021~\cite{nock2021impact}};
    \textcolor[rgb]{0.66,0.81,0.55}{Wu~\textit{et al.}, 2021~\cite{wu2021exploiting}}} \\
\midrule
Privacy \& security & \makecell[c]{
	\textcolor[rgb]{0.92,0.49,0.19}{Xu~\textit{et al.}, 2019~\cite{xu2019achieving}};
    \textcolor[rgb]{0.66,0.81,0.55}{Wang~\textit{et al.}, 2020~\cite{wang2020hybrid}};
    \textcolor[rgb]{0.66,0.81,0.55}{Weng~\textit{et al.}, 2020~\cite{weng2020privacy}}; \\
    \textcolor[rgb]{0.26,0.44,0.76}{Luo~\textit{et al.}, 2021~\cite{luo2021feature}};
    \textcolor[rgb]{0.26,0.44,0.76}{Hou~\textit{et al.}, 2021~\cite{hou2021verifiable}};
    \textcolor[rgb]{0.92,0.49,0.19}{Sun~\textit{et al.}, 2021~\cite{sun2021defending}}} \\
\midrule
Non-IID & \makecell[c]{
    \textcolor[rgb]{0.66,0.81,0.55}{Zhu~\textit{et al.}, 2021~\cite{zhu2021federated}}} \\
\midrule
Application & \makecell[c]{
    \textcolor[rgb]{0.26,0.44,0.76}{Ge~\textit{et al.}, 2021~\cite{ge2021failure}};
    \textcolor[rgb]{0.26,0.44,0.76}{Subramanya~\textit{et al.}, 2021~\cite{subramanya2021centralized}};
    \textcolor[rgb]{0.26,0.44,0.76}{Pfitzner~\textit{et al.}, 2021~\cite{pfitzner2021federated}}; \\
    \textcolor[rgb]{0.66,0.81,0.55}{Liu~\textit{et al.}, 2021~\cite{liu2021federated}}} \\
\midrule
Survey & \makecell[c]{
    \textcolor[rgb]{0.26,0.44,0.76}{Zhu~\textit{et al.}, 2021~\cite{zhu2021from}};
    \textcolor[rgb]{0.66,0.81,0.55}{Lundberg~\textit{et al.}, 2021~\cite{lundberg2021decentralized}}} \\
\bottomrule
\end{tabularx}
\end{table*}

\begin{table*}[!t]
\caption{Main contribution of existing vertical federated learning works.}
\label{tab:contribution}
\centering
\begin{tabularx}{\linewidth}{cccccccc}
\toprule
 & \makecell[c]{Federated learning \\ algorithm} & \makecell[c]{Federated \\ framework} & \makecell[c]{Optimization \\ method} & \makecell[c]{Incentive \\ mechanism} & \makecell[c]{System \\ \& network} & \makecell[c]{Entity \\ alignment} & \makecell[c]{Privacy \\ \& security} \\
\midrule
\textcolor[rgb]{0.26,0.44,0.76}{Gasc{\'o}n~\textit{et al.}, 2017~\cite{gascon2017privacy}} & $\bullet$ &  & & & & & \\
\bottomrule
\end{tabularx}
\end{table*}

A survey of privacy-preserving methods across vertically partitioned data~\cite{vaidya2008survey}

Vertical grid logistic regression (vertigo)~\cite{li2016vertical}

\subsection{Published Articles}
\begin{enumerate}
    % \item Faster Secure Data Mining via Distributed Homomorphic Encryption~\cite{li2020faster}
    % \begin{itemize}
    %     \item propose a novel general distributed HE-based data mining framework towards one step of solving the scaling problem. The main idea is to use the slightly more communication overhead in exchange of shallower computational circuit in HE, so as to reduce the overall complexity.
    % \end{itemize}
    
    % \item Privacy-Preserving Analysis of Vertically Partitioned Data Using Secure Matrix Products~\cite{karr2009privacy}
    %     \begin{itemize}
    %         \item a protocol conducting secure regressions and similar analyses on vertically partitioned data.
    %     \end{itemize}
    
    % \item Privacy Preserving Regression Modelling via Distributed Computation~\cite{sanil2004privacy}
    % \begin{itemize}
    %     \item a linear regression analysis with complete records without disclosing values of their own attributes.
    % \end{itemize}
    
    % \item Privacy-Preserving Multivariate Statistical Analysis: Linear Regression and Classification~\cite{du2004privacy}
    % \begin{itemize}
    %     \item Secure 2-party Multivariate Linear Regression problem and Secure 2-party Multivariate Classification problem.
    % \end{itemize}
    
    % \item Privacy-Preservation for Gradient Descent Methods~\cite{wan2007privacy}
    % \begin{itemize}
    %     \item a preliminary approach to enable privacy preservation in gradient descent methods in general and demonstrate its feasibility in specific gradient descent methods.
    % \end{itemize}
    \item 2003 KDD: Privacy-preserving k-means clustering over vertically partitioned data~\cite{vaidya2003privacy}
   	\begin{itemize}
   		\item K-means for vertically partitioned data	
   	\end{itemize}

    \item 2006 PAKDD: Privacy-preserving svm classification on vertically partitioned data~\cite{yu2006privacy}
   	\begin{itemize}
   		\item Vertical federated SVM for classification problems using secret sharing
   		\item includes both linear and non-linear kernels
   	\end{itemize}

	\item 2008 ACM TKDD: Privacy-preserving decision trees over vertically partitioned data~\cite{vaidya2008privacy}
	\begin{itemize}
		\item vertical federated decision tree
	\end{itemize}
	
	\item 2017 ISCC: Privacy preserving clustering over horizontal and vertical partitioned data~\cite{sheikhalishahi2017privacy}
	\begin{itemize}
		\item hierarchical clustering model for vertically partitioned data
	\end{itemize}

    \item 2017 MLDM: Optimization for Large-Scale Machine Learning with Distributed Features and Observations~\cite{nathan2017optimization}
        \begin{itemize}
            \item doubly distributed optimization algorithms.
        \end{itemize}
    
    \item 2017 Proc. Priv. Enhancing Technol.: Privacy-Preserving Distributed Linear Regression on High-Dimensional Data~\cite{gascon2017privacy}
        \begin{itemize}
            \item hybrid multi-party computation protocol that combines Yao’s garbled circuits with tailored protocols for computing inner products.
        \end{itemize}
        
    \item 2018 DASC/PiCom/DataCom/CyberSciTech: Privacy Preserving Random Decision Tree Classification over Horizontally and Vertically Partitioned Data~\cite{khodaparast2018privacy}
    \begin{itemize}
        \item a framework for constructing Random Decision Trees on horizontally and vertically partitioned dataset.
    \end{itemize}
        
    \item 2018 Journal of Network and Computer Applications: Distributed learning of deep neural network over multiple agents~\cite{gupta2018distributed}
        \begin{itemize}
            \item split learning
            \item health care and finance
            \item shortage of labeled data and computational resources
        \end{itemize}
        
    \item 2019 TIST: Federated Machine Learning: Concept and Applications~\cite{yang2019federated}
        \begin{itemize}
            \item first to introduce the notion of VFL.
        \end{itemize}
    
    \item 2019 Big Data: SecureGBM: Secure Multi-Party Gradient Boosting~\cite{feng2019securegbm}
        \begin{itemize}
            \item “dual- party”secure learning scenario based on two parties — both party own an unique view (i.e., attributes or features) to the sample group of samples while only one party owns the labels.
            \item feature and label data are not allowed to share with others
        \end{itemize}
        
    \item 2019 Big Data: Measure Contribution of Participants in Federated Learning~\cite{wang2019measure}
        \begin{itemize}
            \item fairly calculate the contributions of multiple parties. For Vertical FML we use Shapley Values to calculate the grouped feature importance.
        \end{itemize}
        
    \item 2019 KDD: FDML: A Collaborative Machine Learning Framework for Distributed Features~\cite{hu2019fdml}
        \begin{itemize}
            \item feature distributed machine learning scenario in Tencent.
        \end{itemize}
        
    \item 2020 VLDB: Privacy Preserving Vertical Federated Learning for Tree-based Models~\cite{wu2020privacy}
        \begin{itemize}
            \item propose Pivot, a novel solution for privacy preserving vertical decision tree training and prediction, ensuring that no intermediate information is disclosed other than those the clients have agreed to release.
        \end{itemize}
    
    \item 2020 KDD: Federated Doubly Stochastic Kernel Learning for Vertically Partitioned Data~\cite{gu2020federated}
        \begin{itemize}
            \item use nonlinear learning with kernels instead of traditional data mining and machine learning algorithms in order to train effectively and efficiently.
        \end{itemize}

    \item 2020 FLPI: Federated recommendation systems~\cite{yang2020federated}
        \begin{itemize}
            \item introduce a new notion of federated recommender systems, which is an instantiation of federated learning on decentralized recommendation..
        \end{itemize}
        
    \item 2020 ICARCV: Efficient Asynchronous Vertical Federated Learning via Gradient Prediction and Double-End Sparse Compression~\cite{li2020efficient}
        \begin{itemize}
            \item natural synchronous algorithm, classical vertical federated learning suffers from “Liebig’s Law”
            \item a novel asynchronous vertical federated learning framework with gradient prediction and double- end sparse compression to accelerate the training process and reduce the intermediate result transmission.
        \end{itemize}
        
    \item 2020 TrustCom: Multi-Party Private Set Intersection in Vertical Federated Learning~\cite{lu2020multi}
        \begin{itemize}
            \item new multi-party PSI protocol in VFL which could handle the case that some parties drop out at any point during the execution of protocol
            \item more efficiently compared to the known protocols, especially when the size of dataset gets larger
        \end{itemize}
        
    \item 2020 AAAI: Federated learning for vision-and-language grounding problems~\cite{liu2020federated}
        \begin{itemize}
            \item a federated learning frame- work to obtain various types of image representations from different tasks, which are then fused together to form fine-grained image representations.
            \item include vertical federated learning
        \end{itemize}
        
    \item 2020 Computer Science and Information Systems: A Homomorphic-encryption-based Vertical Federated Learning Scheme for Rick Management~\cite{ou2020homomorphic}
        \begin{itemize}
            \item vertical federated learning system for the for Bayesian machine learning with the homomorphic encryption.
            \item lots of typos.
        \end{itemize}

    \item 2020 FLPI: Large-Scale Kernel Method for Vertical Federated Learning~\cite{dang2020large}
        \begin{itemize}
            \item first approximate the kernel function by the random feature technique.
            \item then federatedly update the predict function by the special designed doubly stochastic gradient without leaking privacy in both data and model.
        \end{itemize}
    
    \item 2021 IEEE Transactions on Neural Networks and Learning Systems: Privacy-Preserving Asynchronous Vertical Federated Learning Algorithms for Multiparty Collaborative Learning~\cite{gu2021privacy}
        \begin{itemize}
            \item first asynchronous federated learning algorithms for vertically partitioned data.
        \end{itemize}
        
    \item 2021 Peer-to-Peer Networking and Applications: Privacy-preserving two-parties logistic regression on vertically partitioned data using asynchronous gradient sharing~\cite{wei2021privacy}
        \begin{itemize}
            \item a protocol using that can complete the logistic regression modeling of vertically partitioned data by asynchronous gradient sharing.
        \end{itemize}
        
    \item 2021 IEEE Intelligent Systems: Secureboost: A lossless federated learning framework~\cite{cheng2021secureboost}
        \begin{itemize}
            \item constructs boosting trees across multiple parties with a carefully designed encryption strategy.
            \item discuss information leakage during the protocol execution and propose ways to provably reduce it.
        \end{itemize}
        
    \item 2021 AAAI: Secure Bilevel Asynchronous Vertical Federated Learning with Backward Updating~\cite{zhang2021secure}
        \begin{itemize}
            \item most existing VFL algorithms are trapped in the synchronous computations, which leads to inefficiency in their real-world applications.
            \item a novel VFL framework integrated with new backward updating mechanism and bilevel asynchronous parallel architecture.
        \end{itemize}
        
    \item 2021 IEEE Internet of Things Journal: Verifiable Privacy-preserving Scheme based on Vertical Federated Random Forest~\cite{hou2021verifiable}
        \begin{itemize}
            \item vertical federated random forest cannot achieve the application level of security, that is, in a system where users are dynamically changing, not only privacy can be preserved, but also data integrity can be verified.
            \item design homomorphic comparison and voting statistics algorithms based on multi-key homomorphic encryption for privacy preservation
            \item propose a multi- client delegated computing verification algorithm to make up for the disadvantage that the above algorithms cannot verify data integrity
        \end{itemize}
        
    \item 2021 ISCAS: Model Optimization Method Based on Vertical Federated Learning~\cite{yang2021model}
        \begin{itemize}
            \item gradient compression, 
            \item only sends important gradient information to reduce communication bandwidth, and only gradients greater than a certain threshold are transmitted.
        \end{itemize}
        
    \item 2021 PAKDD: Vertical Federated Learning for Higher-Order Factorization Machines~\cite{atarashi2021vertical}
        \begin{itemize}
            \item VFL method for higher-order factorization machines
        \end{itemize}
        
    \item 2021 JMIR Medical Informatics: Implementing Vertical Federated Learning Using Autoencoders: Practical Application, Generalizability, and Utility Study~\cite{cha2021implementing}
        \begin{itemize}
            \item autoencoder-based ML model for vertically incomplete data.
        \end{itemize}
        
    \item 2021 SIGMOD: VF2Boost: Very Fast Vertical Federated Gradient Boosting for Cross-Enterprise Learning~\cite{fu2021vf2boost}
        \begin{itemize}
            \item a novel and efficient vertical federated GBDT system.
            \item First, to handle the deficiency caused by frequent mutual-waiting in federated training, we propose a concurrent training protocol to reduce the idle periods.
            \item Second, to speed up the cryptography operations, we analyze the characteristics of the algorithm and propose customized operations.
        \end{itemize}
        
    \item 2021 Wireless Communications and Mobile Computing: Privacy-Preserving Federated Learning Framework with General Aggregation and Multiparty Entity Matching~\cite{zhou2021privacy}
        \begin{itemize}
            \item a privacy-preserving federated learning framework
            \item support the withdrawal of users in vertical federated learning (VFL) scenarios
        \end{itemize}
        
    \item 2021 Journal of Intelligent Manufacturing: Failure prediction in production line based on federated learning: an empirical study~\cite{ge2021failure}
        \begin{itemize}
            \item application on failure prediction in the production line
            \item Federated Support Vector Machine and federated random forest algorithms for the horizontal FL and vertical FL scenarios
        \end{itemize}
        
    \item 2021 The Journal of Supercomputing: Parallelization of the self-organized maps algorithm for federated learning on distributed sources~\cite{kholod2021parallelization}
        \begin{itemize}
            \item parallelizing the Kohonen algorithm used for the federated learning process in a special kind of neural networks— Self-Organizing Maps
            \item reduces the execution time of the algorithm, the network traffic, and the risk of an unauthorized access to the data during their transmission
        \end{itemize}
        
    \item 2021 IEEE TNSM: Centralized and Federated Learning for Predictive VNF Autoscaling in Multi-Domain 5G Networks and Beyond~\cite{subramanya2021centralized}
        \begin{itemize}
            \item application of vertical autoscaling in multi-domain networks
        \end{itemize}
        
    \item 2021 ICASSP: Multi-tier federated learning for vertically partitioned data~\cite{das2021multi}
        \begin{itemize}
            \item a set of silos, each holding a vertical partition of the data. Each silo contains a hub and a set of clients, with the silo’s vertical data shard partitioned horizon- tally across its clients.
            \item new scenario and architecture
        \end{itemize}
        
    \item 2021 TOIT: Federated Learning in a Medical Context: A Systematic Literature Review~\cite{pfitzner2021federated}
        \begin{itemize}
            \item application in medicine
        \end{itemize}
        
    \item 2021 Complex \& Intelligent Systems: From federated learning to federated neural architecture search: a survey~\cite{zhu2021from}
        \begin{itemize}
            \item neural architecture search about VFL
            \item survey
        \end{itemize}
    
    \item 2021 ICML: The Impact of Record Linkage on Learning from Feature Partitioned Data~\cite{nock2021impact}
        \begin{itemize}
            \item there has been so far no formal assessment of the way in which RL errors impact learning models
            \item the first assessment of the problem for supervised learning
        \end{itemize}
        
    \item 2021 ICDE: Feature Inference Attack on Model Predictions in Vertical Federated Learning~\cite{luo2021feature}
        \begin{itemize}
            \item several feature inference attacks in the model prediction stage of VFL.
            \item on LR, DT, NN, RF.
        \end{itemize}
        
    \item 2021 KDD: AsySQN: Faster Vertical Federated Learning Algorithms with Better Computation Resource Utilization~\cite{zhang2021asysqn}
        \begin{itemize}
            \item address the challenges of communication and computation resource utilization
            \item an asynchronous stochastic quasi-Newton (AsySQN) framework for VFL
        \end{itemize}
    
    \item 2021 CIKM: Desirable Companion for Vertical Federated Learning: New Zeroth-Order Gradient Based Algorithm~\cite{zhang2021desirable}
    	\begin{itemize}
    		\item zero-order optimization methods for VFL
    		\item theoretical and empirical guarantee on model privacy and accuracy	
    	\end{itemize}

	\item 2021 CIKM: Large-scale Secure XGB for Vertical Federated Learning~\cite{fang2021large}
		\begin{itemize}
			\item secure computation protocols to train large scale gradient boosting trees	
		\end{itemize}
		
	\item 2022 USENIX Security: Label Inference Attacks Against Vertical Federated Learning~\cite{fu2022label}
	\begin{itemize}
		\item A framework to infer labels of data from VFL. 	
	\end{itemize}

\end{enumerate}

\subsection{Workshop Papers}
\begin{enumerate}
    \item 2019 FL-NeurIPS: A Quasi-Newton Method Based Vertical Federated Learning Framework for Logistic Regression~\cite{yang2019quasi}
        \begin{itemize}
            \item Existing frameworks adopt the first-order stochastic gradient descent algorithm.
            \item propose a quasi-Newton method based vertical federated learning framework for logistic regression under the additively homomorphic encryption scheme.
            \item reduce the number of communication rounds with a little additional communication cost per round.
        \end{itemize}
    
    \item 2019 FL-NeurIPS: A Communication Efficient Collaborative Learning Framework for Distributed Features~\cite{liu2019communication}
        \begin{itemize}
            \item each party conducts multiple local updates before each communication to effectively reduce the number of communication rounds among parties.
        \end{itemize}
    
    \item 2019 FL-IJCAI: Parallel Distributed Logistic Regression for Vertical Federated Learning without Third-Party Coordinator~\cite{yang2019parallel}
        \begin{itemize}
            \item parallel distributed logistic regression for vertical federated learning.
            \item the role of third-party coordinator is removed.
            \item built on the parameter server architecture and aims to speed up the model training via utilizing a cluster of servers in case of large volume of training data.
        \end{itemize}
        
    \item 2019 ICLR AI for social good workshop: Split learning for health: Distributed deep learning without sharing raw patient data~\cite{vepakomma2018split}
        \begin{itemize}
            \item proposes the VFL configurations of SplitNN.
        \end{itemize}
    
    \item 2020 Workshop on Distributed Machine Learning: Accelerating Intra-Party Communication in Vertical Federated Learning with RDMA~\cite{liu2020accelerating}
        \begin{itemize}
            \item transmit data with RDMA for intra-party communication, with no modifications to applications, to improve the network efficiency.
        \end{itemize}

    \item 2020 FL-IJCAI: FedMVT: Semi-supervised Vertical Federated Learning with MultiView Training~\cite{kang2022fedcvt}
        \begin{itemize}
            \item limited overlapping samples.
            \item estimates representations for missing features and predicts pseudo-labels for unlabeled samples.
        \end{itemize}
        
    \item 2020 FL-IJCAI: Asymmetrical Vertical Federated Learning~\cite{liu2020asymmetrically}
        \begin{itemize}
            \item protect sample IDs.
            \item Pohlig-Hellman realization of the adapted private set intersection protocol.
        \end{itemize}

    \item 2020 FL-IJCAI: Achieving Differential Privacy in Vertically Partitioned Multiparty Learning~\cite{xu2019achieving}
        \begin{itemize}
            \item a new framework for differential privacy preserving multiparty learning in the vertically partitioned setting.
        \end{itemize}

    \item 2020 FL-IJCAI: FPGA-Based Hardware Accelerator of Homomorphic Encryption for Efficient Federated Learning~\cite{yang2020fpga}
        \begin{itemize}
            \item an FPGA-based homomorphic encryption framework, aiming to accelerate the training phase in federated learning.
        \end{itemize}
        
    \item 2020 IEEE Globecom Workshop: Vertical Federated Learning Based Privacy-Preserving Cooperative Sensing in Cognitive Radio Networks~\cite{zhang2020vertical}
        \begin{itemize}
            \item vertical federated learning-based cooperative sensing (VFL-CS) scheme
            \item a multi-user deep learning-based FL architecture.
        \end{itemize}
        
    \item 2020 FL-ICML: VAFL: a Method of Vertical Asynchronous Federated Learning~\cite{chen2020vafl}
        \begin{itemize}
            \item each client to run stochastic gradient algorithms without coordination with other clients.
            \item perturbed local embedding to ensure data privacy and improve communication efficiency.
        \end{itemize}
    
    \item 2020 FL-NeurlPS: Label Leakage and Protection in Two-party Split Learning~\cite{li2021label}
        \begin{itemize}
            \item two-party split learning in VFL
            \item prevent the participants’ ground-truth labels from possible leakage
            \item norm attack \& several protection techniques
        \end{itemize}
        
    \item 2020 PPML-NeurlPS: Asymmetric Private Set Intersection with Applications to Contact Tracing and Private Vertical Federated Machine Learning~\cite{angelou2020asymmetric}
        \begin{itemize}
            \item combines traditional DDH-based PSI and PSI-C protocols with compression based on Bloom filters that helps reduce communication in the asymmetric setting.
            \item applications to privacy-preserving contact tracing and machine learning on vertically partitioned data.
        \end{itemize}
    
    \item 2021 DPML-ICLR: Pyvertical: A vertical federated learning framework for multi-headed splitnn~\cite{romanini2021pyvertical}
        \begin{itemize}
            \item a simple dual-headed split neural network for a MNIST classification task, with data samples vertically distributed across two data owners and a data scientist.
        \end{itemize}
        
    \item 2021 FL-ICML: Defending against Reconstruction Attack in Vertical Federated Learning~\cite{sun2021defending}
        \begin{itemize}
            \item how to defend against input leakage attack in Vertical FL.
            \item adversarial training based framework that contains three modules: adversarial reconstruction, noise regularization, and distance correlation minimization.
        \end{itemize}
        
    \item 2021 FL-ICML: Fed-EINI: An Efficient and Interpretable Inference Framework for Decision Tree Ensembles in Federated Learning~\cite{chen2021fed}
        \begin{itemize}
            \item address the interpretability issue in the inference process
            \item allow the dis- closure of feature meaning by concealing decision paths with a communication-efficient secure computation method for inference outputs
        \end{itemize}
    \item 2022 FL-AAAI: MVFLS: Multi-participant Vertical Federated Learning based on Secret Sharing~\cite{shi2022mvfls}
    	\begin{itemize}
    		\item a secret-sharing based vertical federated learning framework for multiple clients
    		\item without a server
    	\end{itemize}
	\item 2021 NFFL-NeurIPS: RVFR: Robust Vertical Federated Learning via Feature Subspace Recovery~\cite{liu2021rvfr}
	\begin{itemize}
		\item A robust VFL approach to training-time backdoor attacks and test-time adversarial attacks
	\end{itemize}
\end{enumerate}

\subsection{arXiv E-prints}
\begin{enumerate}
        
    % \item Privacy-Preserving Asynchronous Federated Learning Algorithms for Multi-Party Vertically Collaborative Learning~\cite{gu2020privacy}
    %     \begin{itemize}
    %         \item first asynchronous federated learning algorithms for vertically partitioned data.
    %     \end{itemize}
        
    \item 2017 arXiv: Private federated learning on vertically partitioned data via entity resolution and additively homomorphic encryption~\cite{hardy2017private}
        \begin{itemize}
            \item add the potentially negative consequences of mistakes in entity resolution.
            \item three-party end-to-end solution in two phases—privacy-preserving entity resolution and federated logistic regression.
        \end{itemize}
        
    \item 2018 arXiv: Entity resolution and federated learning get a federated resolution~\cite{nock2018entity}
        \begin{itemize}
            \item how errors in entity resolution impact learning.
            \item token-based entity resolution algorithm so that it indeed aims at avoiding matching rows belonging to different classes.
        \end{itemize}
        
    \item 2019 arXiv: Interpret federated learning with shapley values~\cite{wang2019interpret}
        \begin{itemize}
            \item model interpretation methods for Federated Learning
            \item measurement of feature importance of vertical Federated Learning
        \end{itemize}
        
    \item 2019 arXiv: Detailed comparison of communication efficiency of split learning and federated learning~\cite{singh2019detailed}
        \begin{itemize}
            \item compare communication efficiencies of two compelling distributed machine learning approaches of split learning and federated learning.
        \end{itemize}
        
    \item 2019 arXiv: Learning privately over distributed features: An ADMM sharing approach~\cite{hu2019learning}
        \begin{itemize}
            \item each party only needs to share a single value for each sample in the training process.
        \end{itemize}
        
    \item 2020 arXiv: The OARF Benchmark Suite: Characterization and Implications for Federated Learning Systems~\cite{hu2020oarf}
        \begin{itemize}
            \item a benchmark suite for federated machine learning systems
            \item includes different data partitioning methods (horizontal, vertical and hybrid)
        \end{itemize}
        
    \item 2020 arXiv: Multi-participant multi-class vertical federated learning~\cite{feng2020multi}
        \begin{itemize}
            \item extending the idea of multi-view learning.
            \item label sharing from its owner to other VFL participants in a privacy-preserving manner.
        \end{itemize}
        
    \item 2020 arXiv: FederBoost: Private Federated Learning for GBDT~\cite{tian2020federboost}
        \begin{itemize}
            \item a framework for private federated learning of GBDT.
            \item for both horizontally and vertically partitioned data.
        \end{itemize}

    \item 2020 arXiv: A Vertical Federated Learning Method for Interpretable Scorecard and Its Application in Credit Scoring~\cite{zheng2020vertical}
        \begin{itemize}
            \item a projected gradient-based method in the vertical federated learning framework for the traditional scorecard.
            \item enables multiple agencies to jointly train an optimized scorecard model in a single training session.
        \end{itemize}
    
    \item 2020 arXiv: Hybrid Differentially Private Federated Learning on Vertically Partitioned Data~\cite{wang2020hybrid}
        \begin{itemize}
            \item builds on the recent advances in VFL-based collaborative training among different organizations which rely on protocols like Homomorphic Encryption (HE) and Secure Multi-Party Computation (MPC) to secure computation and training
            \item analyze how VFL’s intermediate result (IR) can leak private information of the training data during communication.
            \item design a DP-based privacy-preserving algorithm to ensure the data confidentiality of VFL participants.
            \item offers multi-level privacy and adequate privacy budgets.
        \end{itemize}
        
    \item 2020 technical report: Federated-PCA on Vertical-Partitioned Data~\cite{cheung2020federated}
        \begin{itemize}
            \item reduce the dimensionality of sample data
            \item efficiency of subsequent training work
        \end{itemize}
        
    \item 2020 arXiv: Splitnn-driven vertical partitioning~\cite{ceballos2020splitnn}
        \begin{itemize}
            \item SplitNN to facilitate learning from vertically distributed features
        \end{itemize}
        
    \item 2020 arXiv: Privacy-preserving Data Sharing on Vertically Partitioned Data~\cite{tajeddine2020privacy}
        \begin{itemize}
            \item use secure multi-party computation (MPC) to combine the contribution of the data from the parties to train the model.
            \item apply the differentially private variational inference (DPVI) for learning the model
        \end{itemize}
        
    \item 2020 arXiv: Privacy Leakage of Real-World Vertical Federated Learning~\cite{weng2020privacy}
        \begin{itemize}
            \item reverse sum attack and reverse multiplication attack.
            \item effective, evasive, easy.
            \item real-world Secure Computing Frameworks for Vertical Federated Learning.
        \end{itemize}
        
    \item 2020 arXiv: FLFE: A Communication-Efficient and Privacy-Preserving Federated Feature Engineering Framework~\cite{fang2020flfe}
        \begin{itemize}
            \item direct and unlimited multivariate feature transformations will quickly exhaust memory, power, and bandwidth of devices, not to mention the security of information threatened
            \item The framework pre-learns the pattern of the feature to directly judge the usefulness of the transformation on a feature.
        \end{itemize}
    
    \item 2021 arXiv: Vertical Federated Learning without Revealing Intersection Membership~\cite{sun2021vertical}
        \begin{itemize}
            \item Private Set Union (PSU) that allows each party to keep sensitive membership information to itself.
            \item Instead of identifying the intersection of all training samples, our PSU protocol generates the union of samples as training instances.
        \end{itemize}

    \item 2021 arXiv: A Vertical Federated Learning Framework for Horizontally Partitioned Labels~\cite{xia2021vertical}
        \begin{itemize}
            \item labels are horizontally partitioned and the parties only hold partial labels.
        \end{itemize}
        
    \item 2021 arXiv: Vertical federated learning based on DFP and BFGS~\cite{wenjie2021vertical}
        \begin{itemize}
            \item quasi-newton method, BFGS and DFP
        \end{itemize}

    \item 2021 arXiv: Exploiting Record Similarity for Practical Vertical Federated Learning~\cite{wu2021exploiting}
        \begin{itemize}
            \item a novel similarity-based VFL framework.
            \item study the “record linkage” process.
            \item fuzzy matching.
        \end{itemize}
        
    \item 2021 arXiv: Multi-VFL: A Vertical Federated Learning System for Multiple Data and Label Owners~\cite{mugunthan2021multi}
        \begin{itemize}
            \item first to consider the setting where D-data owners (across which features are distributed) and K-label owners (across which labels are distributed) exist.
        \end{itemize}
        
    \item 2021 technical report: Vertical Federated Learning for Emulation of Business-to-Business Applications at the Edge~\cite{Avelar2021VerticalFL}
        \begin{itemize}
            \item illustrate the concepts and provide a practical implementation
            \item more than 8000 times more time to train the VFL model than it takes to train a model locally
        \end{itemize}
        
    \item 2021 arXiv: A Vertical Federated Learning Framework for Graph Convolutional Network~\cite{ni2021vertical}
        \begin{itemize}
            \item a federated GCN learning paradigm for privacy-preserving node classification task under data vertically partitioned setting
        \end{itemize}
        
    \item 2021 arXiv: Federated Learning on Non-IID Data: A Survey~\cite{zhu2021federated}
        \begin{itemize}
            \item Non-IID in vertical federated learning
        \end{itemize}
        
    \item 2021 arXiv: A Federated Learning Framework for Smart Grids: Securing Power Traces in Collaborative Learning~\cite{liu2021federated}
        \begin{itemize}
            \item application in smart grids
            \item two VFL sub-frameworks for collaborative power consumption predictions, based on datasets from two distinct parties.
        \end{itemize}
        
    \item 2021 arXiv: FedV: Privacy-Preserving Federated Learning over Vertically Partitioned Data~\cite{xu2021fedv}
        \begin{itemize}
            \item a framework for secure gradient computation in vertical settings for several widely used ML models such as linear models, logistic regression, and support vector machines.
            \item removes the need for peer-to-peer communication among parties by using functional encryption schemes; this allows FedV to achieve faster training times.
        \end{itemize}
        
    \item 2021 arXiv: Privacy-Preserving Self-Taught Federated Learning for Heterogeneous Data~\cite{chu2021privacy}
        \begin{itemize}
            \item uses unsupervised feature extraction techniques for distributed supervised deep learning tasks
            \item only latent variables are transmitted to other parties for model training, while privacy is preserved by storing the data and parameters of activations, weights, and biases locally.
        \end{itemize}
        
    \item 2021 arXiv: Federated Multi-View Learning for Private Medical Data Integration and Analysis~\cite{che2021federated}
        \begin{itemize}
            \item different sources and views, resulting in heterogeneity and complexity
            \item both V-FedMV and H-FedMV
            \item application in health data
        \end{itemize}
        
    \item 2021 arXiv: Federated Graph Learning--A Position Paper~\cite{zhang2021federated}
        \begin{itemize}
            \item inter- graph FL, intra-graph FL and graph-structured FL
            \item intra-graph is further divided into horizontal and vertical FGL
        \end{itemize}
    
    \item 2021 arXiv: Self-supervised cross-silo federated neural architecture search~\cite{liang2021self}
        \begin{itemize}
            \item Self-supervised Vertical Federated Neural Architecture Search (SS-VFNAS) for automating FL where participants hold feature-partitioned data
        \end{itemize}
        
    \item 2021 master thesis: Decentralized machine learning on massive heterogeneous datasets: A thesis about vertical federated learning~\cite{lundberg2021decentralized}
        \begin{itemize}
            \item current state of the art methods in vertical federated learning, implement the most interesting ones and compare the results in order to draw conclusions of the benefits and drawbacks of the different methods
            \item survey
        \end{itemize}
        
    \item 2021 arXiv: Efficient Batch Homomorphic Encryption for Vertically Federated XGBoost~\cite{xu2021efficient}
        \begin{itemize}
            \item TODO
        \end{itemize}
\end{enumerate}
